# Supplementary material for: The Prompt Artists
Source: arXiv:2303.12253 source file (2023-03-22)
Supplement: Supplementary file 1 [file appendix.tex]

\section{Study Recruiting Ad}

[Study Invitation] Tell us about your experience with Text to Image models!

Tell us about your experience with Text to Image models!
Hello image makers! 
We’re working on the next generation of user interface for Imagen and Parti, and would like to hear more about your experience. Please help us by sharing your typical interaction with the models, what has been great, frustrating, surprising, and disappointing.
We will contact you and schedule the interview individually on your calendar.
	•	Requirements: FTE or intern based in Canada, France, Germany, Israel, Japan, Switzerland, United Kingdom, the United States, with generally reliable internet
	•	Session Dates: Weeks of Aug 1, Aug 8, and Aug 15
	•	Session Length: 45 - 50 minutes
	•	What to bring: THREE prompts of your own creations (they can overlap): One of your most successful prompts, one of your least successful prompts, and one prompt that you're most proud of, and image results to each if you have them)
	•	After completing the study, you will receive 90 massage points or a $60 Perks gift code (note: Google employees may receive a maximum of $65 Perks credit per calendar year)

Here's the Sign-up Link.

\section{Gallery}
\begin{figure}[t]
    % \begin{subfigure}[b]{\textwidth}
        \hspace{\fill} % note: no blank line here
        \includegraphics[width=0.7\linewidth]{\imagepath{AA2 - Whimsical Houses.png}}
        \caption{Example of the prompt ``Audacious and whimsical fantasy house shaped like <object> with windows and doors, <location>''.} 
        \label{fig:more whimsical houses}
    % \end{subfigure}
\end{figure}
